# Supplementary material for: AIMSCheck: Leveraging LLMs for AI-Assisted Review of Modern Slavery Statements Across Jurisdictions
Source: arXiv:2506.01671 source file (2025-06-02)
Supplement: Supplementary file 1 [file Appendix_Mapping.tex]

\section{Legislation Mapping}
\label{sec:appendix_mapping}

\subsubsection{Preprocessing}
The selected statements were downloaded in PDF format, and plain text was extracted from the documents using PyMuPDF \cite{} as well as ABBYY FineReader PDF (a commercial software). Subsequently, the text was split into sentences use the same rule-based process described in AIMS.AU \cite{}.

\tikzstyle{criterion} = [rectangle, draw, text width=5cm, minimum height=1cm, font=\large]
\tikzstyle{question} = [rectangle, draw, text width=7cm, minimum height=1cm, font=\large]
\tikzstyle{example} = [rectangle, draw, text width=12.7cm, minimum height=1cm, font=\large]
\tikzstyle{arrow} = [thick,->,>=stealth]

\begin{figure}[t]
   % \centering
    \hspace*{-8cm}
    \scalebox{0.63}{ 
    \begin{tikzpicture}[node distance=1.4cm and 0.5cm]

    % Column Labels
    \node[align=left, text width=4cm, font=\large] (criterionLabel) at (-3.8, 1.5) {\textbf{AU MSA \\Mandatory Criteria}};
    \node[align=left, text width=9cm, font=\large] (questionLabel) at (4.3, 1.5) {\textbf{AIMS.au Annotation Questions}};
    \node[align=left, text width=13cm, font=\large] (exampleLabel) at (14.4, 1.7) {\textbf{UK MSA Reporting Suggestions, Canadian Act Reporting \\ Obligations and WikiRate Metrics}};

    % Approval and Signature Nodes
    \node[criterion,align=left, fill=green!15]  (approval) at (-3.2, 0) {Statement must be approved by the board.};
    \node[question, align=left,  fill=green!15, right=of approval] (approvalQuestion) {Is the statement approved by the reporting entity’s principal governing body?};
    \node[example, align=left,fill=green!15, right=of approvalQuestion] (approvalExample) {
        \begin{tabular}{l}
            \textbf{UK MSA:} Approval from board of directors (or equivalent management \\ body).\\
            \textbf{CA Act:} Approval by the organization’s governing body.\\
            \textbf{WikiRate:} Statement Approval
        \end{tabular}
    };

    \node[criterion,align=left, below=of approval,  fill=green!15]  (signature) {Signed by a responsible \\member of the organization.};
    \node[question, align=left, fill=green!15,right=of signature] (signatureQuestion) {Is the statement signed by a responsible member of the reporting entity?};
    \node[example,align=left, fill=green!15, right=of signatureQuestion] (signatureExample) {
        \begin{tabular}{l}
            \textbf{UK MSA:} Signature from a director (or equivalent) or designated \\member.\\
            \textbf{CA Act:} Signature of one or more members of the governing body of \\each approving entity.\\
            \textbf{WikiRate:} Statement Signing
        \end{tabular}
    };

    % Criterion Nodes
    \node[criterion, align=left, below=of signature, fill=red!15] (criterion1) {Mandatory Criterion 1: The statement must clearly identify the reporting entity.};
    \node[question, align=left, fill=red!15,right=of criterion1] (question1) {Does the statement clearly identify the reporting entity?};
    \node[example,align=left, fill=red!15, right=of question1] (example1) {
        \begin{tabular}{l}
            \textbf{UK MSA:} N/A\\
            \textbf{CA Act:} N/A\\
            \textbf{WikiRate:} N/A
        \end{tabular}
    };

    \node[criterion, align=left,fill=green!15,below=1.1cm of criterion1] (criterion2) {Mandatory Criterion 2: Describe the entity’s structure, operations, and supply chains.};
    \node[question,align=left,fill=green!15, right=of criterion2] (question2) {
        Does the entity describe its structure?\\
        Does the entity describe its operations?\\
        Does the entity describe its supply chains?
    };
    \node[example,align=left,fill=green!15,  right=of question2] (example2) {
        \begin{tabular}{l}
            \textbf{UK MSA:} Organization’s structure, business, and supply chains.\\
            \textbf{CA Act:} Description of the organization’s structure, activities, and \\supply chains.\\
            \textbf{WikiRate:} Organizational Structure and Operations, Supply chain \\disclosure
        \end{tabular}
    };

    \node[criterion,fill=green!15,below=1.1cm of criterion2] (criterion3) {Mandatory Criterion 3: Describe the risks of modern slavery practices in operations and supply chains.};
    \node[question, align=left,fill=green!15, right=of criterion3] (question3) {Does the entity describe its modern slavery risks?};
    \node[example,align=left,fill=green!15, fill=green!15,right=of question3] (example3) {
        \begin{tabular}{l}
            \textbf{UK MSA:} Risk assessment and management.\\
            \textbf{CA Act:} Description of business and supply chain risks, steps taken \\ to assess and manage them.\\
            \textbf{WikiRate:}Identification of Risks, Incidents Identified
        \end{tabular}
    };

    \node[criterion, align=left, fill=yellow!15, below=of criterion3] (criterion4) {Mandatory Criterion 4: Describe the actions taken to assess and address these risks, including due diligence and remediation processes };
    \node[question,align=left, fill=yellow!15, right=of criterion4] (question4) {

          Does the entity describe actions to  \\ identify, assess, and mitigate modern slavery risks?\\
        Does it describe remediation actions?

    };
    \node[example,align=left, fill=yellow!15, right=of question4] (example4) {
        \begin{tabular}{l}
            \textbf{UK MSA:} Policies on slavery and human trafficking, Due diligence \\processes, \\ Risk assessment and management steps, Training for staff.\\
            \textbf{CA Act:} Policies and due diligence processes on forced labor and \\child labor, \\ Risk assessment and mitigation steps, Training for employees. \\ 
            \textbf{WikiRate:} Policy, Whistleblowing mechanism, \\ Risk management, Risk assessment, Training
        \end{tabular}
    };

    \node[criterion,align=left,fill=green!15, below=of criterion4] (criterion5) {Mandatory Criterion 5: Describe how the reporting entity assesses the effectiveness of actions being taken.};
    \node[question, align=left,fill=green!15,right=of criterion5] (question5) {Does the entity describe how it assesses the effectiveness of actions?};
    \node[example,align=left, fill=green!15, right=of question5] (example5) {
        \begin{tabular}{l}
            \textbf{UK MSA:} Effectiveness of anti-slavery measures, measured against \\relevant indicators.\\
            \textbf{CA Act:} Description of how effectiveness is assessed in ensuring \\no forced or child labor is used. \\
            \textbf{WikiRate:} Performance Indicators
        \end{tabular}
    };

    \node[criterion,align=left,fill=red!15, below=of criterion5] (criterion6) {Criterion 6: Describe the process of consultation with any entities the reporting entity owns or controls };
    \node[question, align=left,fill=red!15,right=of criterion6] (question6) {Does the entity describe consultation processes with entities it owns or controls?};
    \node[example,align=left, fill=red!15, right=of question6] (example6) {
        \begin{tabular}{l}
            \textbf{UK MSA:} N/A  \\
            \textbf{CA Act:} N/A\\
            \textbf{WikiRate:} N/A 
        \end{tabular}
    };

     \node[criterion,align=left, fill=red!15,below=of criterion6] (criterion7) {Mandatory Criterion 7: Any other relevant information};
    \node[question, align=left, fill=red!15,right=of criterion7] (question7) {N/A};
    \node[example,align=left, fill=red!15, right=of question7] (example7) {
        \begin{tabular}{l}
            \textbf{UK MSA:} N/A  \\
            \textbf{CA Act:} Measures to remediate income loss of vulnerable families \\ due to anti-slavery actions.\\
            \textbf{WikiRate:} Mineral sourcing, Living wage in supply chains, \\Agency workers, Artisanal and Small Scale Mining, \\Business Performance Indicators, Collaborations and Memberships, \\Forced overtime, Migrant Workers, Purchasing Practices, \\State-imposed Forced Labour, Workers Engagement, Historic Record 
        \end{tabular}
    };   

    % Arrows
    \draw[arrow] (approval.east) -- (approvalQuestion.west);
    \draw[arrow] (approvalQuestion.east) -- (approvalExample.west);

    \draw[arrow] (signature.east) -- (signatureQuestion.west);
    \draw[arrow] (signatureQuestion.east) -- (signatureExample.west);

    \draw[arrow] (criterion1.east) -- (question1.west);
    \draw[arrow] (question1.east) -- (example1.west);

    \draw[arrow] (criterion2.east) -- (question2.west);
    \draw[arrow] (question2.east) -- (example2.west);

    \draw[arrow] (criterion3.east) -- (question3.west);
    \draw[arrow] (question3.east) -- (example3.west);

    \draw[arrow] (criterion4.east) -- (question4.west);
    \draw[arrow] (question4.east) -- (example4.west);

    \draw[arrow] (criterion5.east) -- (question5.west);
    \draw[arrow] (question5.east) -- (example5.west);

    \draw[arrow] (criterion6.east) -- (question6.west);
    \draw[arrow] (question6.east) -- (example6.west);

    \draw[arrow] (criterion7.east) -- (question7.west);
    \draw[arrow] (question7.east) -- (example7.west);

    \end{tikzpicture}
    }

 \caption {Mapping between the AIMS.au Annotations Questions and the AU, UK and CA Acts Reporting Criteria. \textcolor{green}{Green:} perfect alignment, \textcolor{yellow}{Yellow:}partial match, \textcolor{red}{Red:} no overlap, requiring re-annotation.}
 \label{fig:modern_slavery_flowchart}
\end{figure}

\section{Appendix}

\subsection{Appendix A}
\label{appendix_mapping}
\begin{table}[h]
\label{mappingtable}
\centering
\resizebox{\textwidth}{!}{%
\begin{tabular}{|p{6.5cm}|p{5.5cm}|p{6.5cm}|}
\hline
\textbf{AU MSA Mandatory Criteria} & \textbf{UK MSA} & \textbf{Canadian Act} \\
\hline
Identify the reporting entity 
& N/A 
& N/A \\
\hline
Describe the reporting entity’s structure, operations and supply chains 
& Organisational structure, its business and its supply chains.
& Its structure, activities and supply chains. \\
\hline
Describe the risks of modern slavery practices in the operations and supply chains of the reporting entity and any entities it owns or controls
& Assessing and managing risk.
& The parts of its business and supply chains that carry a risk of forced labour or child labour being used and the steps it has taken to assess and manage that risk. \\
\hline
Describe the actions taken by the reporting entity and any entities it owns or controls to assess and address these risks, including due diligence and remediation processes
& Organisational policies, due diligence in relation to modern slavery (including approach to remediation), assessing and managing risk, training.
& Its policies and due diligence processes in relation to forced labour and child labour; any measures taken to remediate any forced labour or child labour; the training provided to employees on forced labour and child labour. \\
\hline
Describe how the reporting entity assesses the effectiveness of these actions
& Monitoring and evaluation (understanding and demonstrating effectiveness).
& How the entity assesses its effectiveness in ensuring that forced labour and child labour are not being used in its business and supply chains. \\
\hline
Describe the process of consultation with any entities the reporting entity owns or controls (a joint statement must also describe consultation with the entity giving the statement)
& N/A 
& N/A \\
\hline
Provide any other relevant information
& N/A 
& Any measures taken to remediate the loss of income to the most vulnerable families that results from any measure taken to eliminate the use of forced labour or child labour in its activities and supply chains. \\
\hline
Statement must be approved by the board.
& Approval from board of directors (or equivalent management body). 
& Approval by the organization’s governing body. \\
\hline
Signed by a responsible member of the organization.
& Signature from director or designated member. 
& Signature from members of governing body. \\
\hline
\end{tabular}%
}
\caption{Mapping between the AU, UK, and CA Acts Reporting Criteria.}
\label{tab:legislation_mapping}
\end{table}
